# Supplementary material for: Deep Global Registration
Source: arXiv:2004.11540 source file (2020-05-08)
Supplement: Supplementary file 1 [file scene_wise_5cm.tex]

\begin{table}[h]
\centering
\small
\caption{Scene-wise statistics for our method on 3DMatch test set.}\label{tab:abalation_weighted}
\resizebox{0.50\linewidth}{!}{
\begin{tabular}{l||c|c|c|c}
    \hline
    Scene & Recall & TE (cm) & RE (deg) & Time (s) \\
    \hline
    Kitchen & 94.5\% & 6.30  & 2.25  & 0.70\\
    Home1   & 89.7\% & 7.78  & 2.34  & 0.66\\
    Home2   & 77.9\% & 8.31  & 3.49  & 0.62\\
    Hotel1  & 92.9\% & 7.22  & 2.38  & 0.74\\
    Hotel2  & 85.5\% & 6.49  & 2.43  & 0.72\\
    Hotel3  & 79.6\% & 7.13  & 2.44  & 0.68\\
    Study   & 69.9\% & 11.59 & 3.23  & 0.73\\
    Lab     & 72.7\% & 8.36  & 2.04  & 0.73\\
    \hline
\end{tabular}
}
\end{table}
