# Supplementary material for: Deep Global Registration
Source: arXiv:2004.11540 source file (2020-05-08)
Supplement: Supplementary file 2 [file weight_ablation.tex]

\begin{table}[h]
\centering
\small
\caption{Registration results w/ and w/o Weighted Procrustes, with different voxel sizes.}\label{tab:abalation_weighted}
\resizebox{0.55\linewidth}{!}{
\begin{tabular}{l||c|c|c|c}
    \hline
     & Recall & TE (cm) & RE (deg) & Time (s) \\
    \hline
    2.5cm-weighted           & {82.4}\% & {7.61} & {2.44} & 2.24 \\    
    2.5cm-nonweighted       & 81.9\% & \textbf{7.21} & \textbf{2.39} & 2.27 \\ 
    \hline
    5cm-weighted         & \textbf{85.2}\% & 7.73 & 2.58 & 0.70 \\
    5cm-nonweighted      & 85.0\% & 7.44 & 2.42 & \textbf{0.69} \\   \hline
\end{tabular}
}
\end{table}
